# Supplementary material for: SoK: Safer Digital-Safety Research Involving At-Risk Users
Source: arXiv:2309.00735 source file (2023-09-01)
Supplement: Supplementary file 1 [file 00-appendix.tex]

\section{Paper count and distribution.}
\label{appendix:paper-count}
\begin{table}[ht]
\begin{tabular}{l|lllllll}
Venue                     & 2015 & 2016 & 2017 & 2018 & 2019 & 2020 & 2021 \\ \hline
% \textit{\textbf{CCS}}     & 0    & 1    & 0   & 0   & 0   & 0   & 0   \\
\textit{\textbf{CHI}}     & 1    & 6    & 12   & 14   & 15   & 17   & 11   \\
\textit{\textbf{COMPASS}} & 0    & 0    & 0    & 1    & 0    & 0   & 4    \\
\textit{\textbf{CSCW}}    & 0    & 1    & 13    & 2    & 5    & 2   & 11    \\
\textit{\textbf{IEEE S\&P}}    & 0    & 0    & 0    & 3    & 0    & 1   & 0    \\
\textit{\textbf{PoPETS}}  & 0    & 2    & 2    & 2    & 2    & 1   & 1    \\
\textit{\textbf{SOUPS}}   & 1    & 2    & 5    & 1    & 2    & 5   & 1    \\
\textit{\textbf{USENIX}}  & 1    & 0    & 1    & 0    & 3    & 4    & 5   \\ \hline
\end{tabular}
\caption{Counts of papers related to digital-safety research with at-risk groups at selected \\ venues in HCI and S\&P from 2015-2021.}
\label{tab:venue-breakdown}
\end{table}

\section{Methods used in the digital safety corpus.}
\label{appendix:methods}
\begin{table}[!h]
\resizebox{\columnwidth}{!}{%
\begin{tabular}{lclclc}
\textbf{Method Category} & \textbf{Count} &  &  &  &  \\ \hline
\textbf{Interview} & 89 & \textbf{Creativity-Based Approaches} & 25 & \textbf{Tool Evaluation} & 33 \\ \cline{1-1} \cline{3-3} \cline{5-5}
Semi-Structured Interview & 76 & Co-Design Sessions & 3 & Testing Design Mockups & 4 \\
In-Depth Interview & 4 & Illustration & 5 & Tool Evaluation & 23 \\
Structured Interview & 6 & Card Sorting Exercise & 2 & Speak-Aloud Walkthroughs & 1 \\
Narrative Interview & 2 & Design Workshop & 14 & Artefact Analysis & 1 \\
\textbf{Survey} & 53 & \textbf{Measurement Studies} & 25 & Personal device examination & 1 \\ \cline{1-1} \cline{3-3}
Online Survey & 30 & Social Media Scrape & 13 & Log Analysis & 3 \\
Pre-Deployment survey & 4 & Web scrape & 3 & \textbf{Observation-Based} & 19 \\ \cline{5-5}
Post-Deployment Survey & 10 & Measurement Pipeline & 3 & Ethnography & 7 \\
Demographic survey & 9 & App Audit & 6 & Online Ethnography & 2 \\
\textbf{Group Discussion} & 20 & \textbf{Document-Based} & 8 & Field Observations & 10 \\ \cline{1-1} \cline{3-3}
Focus Groups & 17 & Diary Study & 4 & \textbf{Critical Analysis} & 5 \\ \cline{5-5}
Focused Group Discussions & 3 & Document Analysis & 4 & Case study-based & 5
\end{tabular}%
}
\caption{\label{tab:method-breakdown}Data collection approaches used in digital-safety research with and about at-risk groups. We note that individual papers may use more than one method.}
\end{table}
